# Supplementary material for: Reduced Tensor Product on the Drinfeld Center
Source: arXiv:2004.09611 source file (2021-12-26)
Supplement: Supplementary file 1 [file appendix.tex]

\section{Appendix}

Testing
\begin{equation}
\label{e:def_H}
%%% \hA stuff %%%%%%%%%%%%%%%%%%%%%%%%%%%%%%%%%%%%%%%%%%%
\begin{tikzpicture}
\node at (0,2) {$\hA$};
\node at (0,1.2) {$Y$};
\node at (0,-1.2) {$Y'$};
\node[small_morphism] (ph) at (0,0) {$\vphi$};
\draw (ph) -- (0,-1);
\draw (ph) -- (0,1);
\draw (ph) -- (-0.5,0.5) node[left] {$A$};
\draw (ph) -- (0.5,-0.5) node[right] {$A$};
\end{tikzpicture}
%%%%%%%%%%%%%%%%%%%%%%%%%%%%%%%
\begin{tikzpicture}
\node at (0,0) {$\mapsto$};
\node at (0,-1.2) {$\mapsto$};
\node at (0,1.2) {$\mapsto$};
\node at (0,2) {$\overset{H}{\simeq}$};
\end{tikzpicture}
%%%%%%%%%%%%%%%%%%%%%%%%%%%%%%%%%%%%%%%%%%%%%%%%%%%%%%%%%%
\begin{tikzpicture}
\node at (0,2) {$\hCYA$};
\tikzmath{
  \toprow = 0.7;
  \bottom = -0.7;
  \midrow = 0;
  \bigx = 1; %size of big ellipse
  \bigy = 0.2;
  \smlx = 0.5;
  \smly = 0.1;
  \medx = 0.75;
  \medy = 0.15;
}
%%%%% the objects, top and bottom Annulus
\draw (0,1.2) ellipse (\bigx cm and \bigy cm);
\draw (0,1.2) ellipse (\smlx cm and \smly cm);
\node[dotnode, label={[shift={(0,0.1)}] \small $Y$}] at (-\medx,1.2) {};
\draw (0,-1.2) ellipse (\bigx cm and \bigy cm);
\draw (0,-1.2) ellipse (\smlx cm and \smly cm);
\node[dotnode, label={[shift={(0,-0.6)}] \small $Y'$}] at (-\medx,-1.2) {};
%%%%%%%%%%%%%%%%%%%%%%%%%%%%%%%%%%%%%%%%%%%%%%%%%%%%
%%% the graph %%%%%%%%%%%%%%%%%%%%%%%%%%%%%%%%%%%%%%
%% bottom ellipse
\draw (0,\bottom) ellipse (\bigx cm and \bigy cm);
%\draw (0,0) ellipse (0.5cm and 0.25cm); don't want to get covered
%% back half of graph
\draw (\medx,\midrow) arc(0:180:\medx cm and \medy cm);
%% inner vertical lines
\draw[overline={1.5}] (-0.5,\bottom) -- (-0.5,\toprow);
\draw[overline={1.5}] (0.5,\bottom) -- (0.5,\toprow);
\draw (0,\bottom) ellipse (\smlx cm and \smly cm); %bottom inner ellipse
%% graph
\node[dotnode] (top) at (-\medx,\toprow) {}; %% make label later because of overline
\node[dotnode] (bottom) at (-\medx,\bottom) {};
\draw[overline={1.5}, midarrow_rev]
  (\medx,\midrow) arc(0:-180:\medx cm and \medy cm)
  node[pos=0.5, below] {\tiny $A$};
\draw[overline={1},midarrow={0.3},midarrow={0.9}]
  (top) -- (bottom);
\node[small_morphism] at (-\medx,\midrow) {\tiny $\ph$};
%% top ellipse
\draw[overline={1}] (0,\toprow) ellipse (\bigx cm and \bigy cm);
\draw (0,\toprow) ellipse (\smlx cm and \smly cm);
%% vertical lines
\draw (-1,\bottom) -- (-1,\toprow);
\draw (1,\bottom) -- (1,\toprow);
%% labels Y, Y'
\node[style={fill=white,circle,inner sep=0pt,
  minimum size=0pt, scale=0.8}] at (-0.95,0.4) {\tiny $Y$};
\node[style={fill=white,circle,inner sep=0pt,
  minimum size=0pt, scale=0.8}] at (-0.95,-0.4) {\tiny $Y'$};
\node at (-0.6,1.2) {\tiny $p$};
\node at (-0.6,-1.2) {\tiny $p$};
\end{tikzpicture}
%%%%%%%%%%%%%%%%%%%%%%%%%%%%%%%%%%%%%%%%%%%%%%%%%%%%%%%%%%A
%%%%%%%%%%%%%%%%%%%%%%%%%%%%%%%%%%%%%%%%%%%%%%%%%%%%%%%%%%
\end{equation}
\begin{equation*}
%%% Ann %%%%%%%%%%%%%%%%%%%%%%%%%%%%%%%%%%%%%%%%%%%%%%%%
\begin{tikzpicture}
\tikzmath{
  \toprow = 0.7;
  \bottom = -0.7;
  \midrow = 0;
  \bigx = 1; %size of big ellipse
  \bigy = 0.2;
  \smlx = 0.5;
  \smly = 0.1;
  \medx = 0.75;
  \medy = 0.15;
}
%% bottom ellipse
\draw (0,\bottom) ellipse (\bigx cm and \bigy cm);
%\draw (0,0) ellipse (0.5cm and 0.25cm); don't want to get covered
%% back half of graph
\draw (\medx,\midrow) arc(0:180:\medx cm and \medy cm);
%% inner vertical lines
\draw[overline={1.5}] (-0.5,\bottom) -- (-0.5,\toprow);
\draw[overline={1.5}] (0.5,\bottom) -- (0.5,\toprow);
\draw (0,\bottom) ellipse (\smlx cm and \smly cm); %bottom inner ellipse
%% graph
\node[dotnode] (top) at (-\medx,\toprow) {}; %% make label later because of overline
\node[dotnode] (bottom) at (-\medx,\bottom) {};
\draw[overline={1.5}, midarrow_rev]
  (\medx,\midrow) arc(0:-180:\medx cm and \medy cm)
  node[pos=0.5, below] {\tiny $A$};
\draw[overline={1},midarrow={0.3},midarrow={0.85}]
  (top) -- (bottom);
\node at (-0.6,0.35) {\tiny $Y$};
\node at (-0.6,-0.35) {\tiny $Y'$};
\node[small_morphism] at (-\medx,\midrow) {\tiny $\ph$};
%% top ellipse
\draw[overline={1}] (0,\toprow) ellipse (\bigx cm and \bigy cm);
\draw (0,\toprow) ellipse (\smlx cm and \smly cm);
%% vertical lines
\draw (-1,\bottom) -- (-1,\toprow);
\draw (1,\bottom) -- (1,\toprow);
\end{tikzpicture}
%%%%%%%%%%%%%%%%%%%%%%%%%%%%%%%%%%%%%%%%%%%%%%%%%%%%%%%%%%A
\end{equation*}

\comment{
\begin{equation*}
%%% Ann %%%%%%%%%%%%%%%%%%%%%%%%%%%%%%%%%%%%%%%%%%%%%%%%
\begin{tikzpicture}
\tikzmath{
  \toprow = 0.8;
  \bottom = -0.8;
  \midrow = 0.2;
  \bigx = 1; %size of big ellipse
  \bigy = 0.2;
  \smlx = 0.5;
  \smly = 0.1;
  \medx = 0.75;
  \medy = 0.15;
}
%% bottom ellipse
\draw (0,\bottom) ellipse (\bigx cm and \bigy cm);
%\draw (0,0) ellipse (0.5cm and 0.25cm); don't want to get covered
%% back half of graph
\draw (\medx,\midrow) arc(0:180:\medx cm and \medy cm);
%% inner vertical lines
\draw[overline={1.5}] (-0.5,\bottom) -- (-0.5,\toprow);
\draw[overline={1.5}] (0.5,\bottom) -- (0.5,\toprow);
\draw (0,\bottom) ellipse (\smlx cm and \smly cm); %bottom inner ellipse
%% gray arrows indicate flipping operation
\draw[gray,overline={1},->] (-0.4,-0.55)
  to[out=60,in=-60] (-0.4,0.55);
\draw[gray,overline={1},->] (0.4,-0.55)
  to[out=120,in=-120] (0.4,0.55);
\draw[gray,->] (-1.1,0.55)
  to[out=-120,in=120] (-1.1,-0.55);
\draw[gray,->] (1.1,0.55)
  to[out=-60,in=60] (1.1,-0.55);
%% graph
\node[dotnode] (top) at (-\medx,\toprow) {}; %% make label later because of overline
\node[dotnode, label={[shift={(0.,-0.6)}] \small $Y'$}] (bottom) at (-\medx,\bottom) {};
\draw[overline={1.5}, midarrow_rev]
  (\medx,\midrow) arc(0:-180:\medx cm and \medy cm)
  node[pos=0.5, below] {\tiny $A$};
\draw[overline={1}] (top) -- (bottom);
\node[small_morphism] at (-\medx,\midrow) {\tiny $\ph$};
%% top ellipse
\draw[overline={1}] (0,\toprow) ellipse (\bigx cm and \bigy cm);
\draw (0,\toprow) ellipse (\smlx cm and \smly cm);
%% vertical lines
\draw (-1,\bottom) -- (-1,\toprow);
\draw (1,\bottom) -- (1,\toprow);
%% node label
\node[label={\small $Y^*$}] at (-\medx,\toprow) {};
\end{tikzpicture}
%%%%%%%%%%%%%%%%%%%%%%%%%%%%%%%%%%%%%%%%%%%%%%%%%%%%%%%%%%
\mapsto
%%%%%%%%%%%%%%%%%%%%%%%%%%%%%%%%%%%%%%%%%%%%%%%%%%%%%%%%%%
\begin{tikzpicture}
\tikzmath{
  \toprow = 0.8;
  \bottom = -0.8;
  \midrow = -0.2;
  \bigx = 1; %size of big ellipse
  \bigy = 0.2;
  \smlx = 0.5;
  \smly = 0.1;
  \medx = 0.75;
  \medy = 0.15;
}
%% bottom ellipse
\draw (0,\bottom) ellipse (\bigx cm and \bigy cm);
%\draw (0,0) ellipse (0.5cm and 0.25cm); don't want to get covered
%% back half of graph
\draw (\medx,\midrow) arc(0:180:\medx cm and \medy cm);
%% inner vertical lines
\draw[overline={1.5}] (-0.5,\bottom) -- (-0.5,\toprow);
\draw[overline={1.5}] (0.5,\bottom) -- (0.5,\toprow);
\draw (0,\bottom) ellipse (\smlx cm and \smly cm); %bottom inner ellipse
%% graph
\node[dotnode] (top) at (-\medx,\toprow) {}; %% make label later because of overline
\node[dotnode, label={[shift={(0,-0.6)}] \small $Y^*$}] (bottom) at (-\medx,\bottom) {};
\draw[overline={1.5}, midarrow_rev]
  (\medx,\midrow) arc(0:-180:\medx cm and \medy cm)
  node[pos=0.5, above] {\tiny $A$};
\draw[overline={1}] (top) -- (bottom);
\node[small_morphism] at (-\medx,\midrow)
  {\tiny $\rotatebox[origin=c]{180}{\(\ph\)}$};
%% top ellipse
\draw[overline={1}] (0,\toprow) ellipse (\bigx cm and \bigy cm);
\draw (0,\toprow) ellipse (\smlx cm and \smly cm);
%% vertical lines
\draw (-1,\bottom) -- (-1,\toprow);
\draw (1,\bottom) -- (1,\toprow);
%% node label
\node[label={\small $Y'$}] at (-\medx,\toprow) {};
\end{tikzpicture}
%%%%%%%%%%%%%%%%%%%%%%%%%%%%%%%%%%%%%%%%%%%%%%%%%%%%%%%%%%
=
%%%%%%%%%%%%%%%%%%%%%%%%%%%%%%%%%%%%%%%%%%%%%%%%%%%%%%%%%%
\begin{tikzpicture}
\tikzmath{
  \toprow = 0.8;
  \bottom = -0.8;
  \midrow = 0;
  \bigx = 1; %size of big ellipse
  \bigy = 0.2;
  \smlx = 0.5;
  \smly = 0.1;
  \medx = 0.75;
  \medy = 0.15;
}
%% bottom ellipse
\draw (0,\bottom) ellipse (\bigx cm and \bigy cm);
%\draw (0,0) ellipse (0.5cm and 0.25cm); don't want to get covered
%% back half of graph
\draw (\medx,\midrow) arc(0:180:\medx cm and \medy cm);
%% inner vertical lines
\draw[overline={1.5}] (-0.5,\bottom) -- (-0.5,\toprow);
\draw[overline={1.5}] (0.5,\bottom) -- (0.5,\toprow);
\draw (0,\bottom) ellipse (\smlx cm and \smly cm); %bottom inner ellipse
%% graph
\node[dotnode] (top) at (-\medx,\toprow) {}; %% make label later because of overline
\node[dotnode, label={[shift={(0.,-0.6)}] \small $Y^*$}]
  (bottom) at (-\medx,\bottom) {};
\draw[overline={1}]
  (top) .. controls +(down:0.5cm) and +(up:0.3cm) ..
  (-0.95,\midrow) .. controls +(down:0.3cm) and +(down:0.3cm) ..
  (-\medx,\midrow) .. controls +(up:0.3cm) and +(up:0.3cm) ..
  (-0.55,\midrow) .. controls +(down:0.3cm) and +(up:0.5cm) .. (bottom);
\draw[overline={1.5}, midarrow_rev]
  (\medx,\midrow) arc(0:-180:\medx cm and \medy cm)
  node[pos=0.5, below] {\tiny $A$};
\node[small_morphism] at (-\medx,\midrow) {\tiny $\ph$};
%% top ellipse
\draw[overline={1}] (0,\toprow) ellipse (\bigx cm and \bigy cm);
\draw (0,\toprow) ellipse (\smlx cm and \smly cm);
%% vertical lines
\draw (-1,\bottom) -- (-1,\toprow);
\draw (1,\bottom) -- (1,\toprow);
%% node label
\node[label={\small $Y'$}] at (-\medx,\toprow) {};
\end{tikzpicture}
\end{equation*}
}

\comment{
\[
\begin{tikzpicture}%[scale=0.8]
\draw (-2.5,1) ellipse (2cm and 0.4cm);
\draw (-2.5,1) ellipse (1.8 cm and 0.36cm);
\draw (-2.5,1) ellipse (1cm and 0.2cm);
\draw (-2.5,1) ellipse (0.8cm and 0.16cm);
\draw (2.5,1) ellipse (2cm and 0.4cm);
\draw (2.5,1) ellipse (1.8 cm and 0.36cm);
\draw (2.5,1) ellipse (1cm and 0.2cm);
\draw (2.5,1) ellipse (0.8cm and 0.16cm);
\draw (0,0) ellipse (2cm and 0.4cm);
\draw (0,0) ellipse (1.8 cm and 0.36cm);
\draw (0,0) ellipse (1cm and 0.2cm);
\draw (0,0) ellipse (0.8cm and 0.16cm);
\draw (0,-1) ellipse (1.5cm and 0.3cm);
\draw (0,-1) ellipse (1.3cm and 0.26cm);
%%%%%% top half
%% vertical lines
\draw (-4.5,1)
  .. controls +(down:0.4cm) and +(up:0.2cm) .. (-2,0);
\draw (4.5,1)
  .. controls +(down:0.4cm) and +(up:0.2cm) .. (2,0);
\draw (-4.3,1)
  .. controls +(down:0.4cm) and +(up:0.2cm) .. (-1.8,0);
\draw (4.3,1)
  .. controls +(down:0.4cm) and +(up:0.2cm) .. (1.8,0);
\draw (-3.5,1)
  .. controls +(down:0.4cm) and +(up:0.2cm) .. (-1,0);
\draw (3.5,1)
  .. controls +(down:0.4cm) and +(up:0.2cm) .. (1,0);
\draw (-3.3,1)
  .. controls +(down:0.4cm) and +(up:0.2cm) .. (-0.8,0);
\draw (3.3,1)
  .. controls +(down:0.4cm) and +(up:0.2cm) .. (0.8,0);
%% inside
\draw (-0.5,1)
  .. controls +(down:0.3cm) and +(down:0.3cm) .. (0.5,1);
\draw (-0.7,1)
  .. controls +(down:0.35cm) and +(down:0.35cm) .. (0.7,1);
\draw (-1.5,1)
  .. controls +(down:0.5cm) and +(down:0.5cm) .. (1.5,1);
\draw (-1.7,1)
  .. controls +(down:0.55cm) and +(down:0.55cm) .. (1.7,1);
%%%%%%%%%%%%%%% bottom half
\draw (-2,0) to[out=-90,in=90] (-1.5,-1);
\draw (-0.8,0) to[out=-90,in=90] (-1.3,-1);
\draw (2,0) to[out=-90,in=90] (1.5,-1);
\draw (0.8,0) to[out=-90,in=90] (1.3,-1);
\draw (-1.8,0)
  .. controls +(down:0.5cm) and +(down:0.5cm) .. (-1,0);
\draw (1.8,0)
  .. controls +(down:0.5cm) and +(down:0.5cm) .. (1,0);
%%%%%%%%%%%%%%%% gray curve for projector
\draw[gray]
(0,0.75) .. controls +(left:0.5cm) and +(left:0.2cm) ..
(-0.3,-0.6) .. controls +(right:0.1cm) and +(left:0.2cm) ..
(0,0.6) .. controls +(right:0.1cm) and +(left:0.1cm) ..
(0.2,-0.1) .. controls +(right:0.2cm) and +(right:0.2cm) ..
(0,0.75);
%% labels
\node at (-4.7,1) {$\overline{\VV}$};
\node at (-3.7,1) {$\overline{\WW}$};
\node at (0.3,1.05) {$\overline{\VV}'$};
\node at (1.3,1.05) {$\overline{\WW}'$};
\end{tikzpicture}
\]
\[
\begin{tikzpicture}%[scale=0.8]
\draw (-2.5,1) ellipse (2cm and 0.4cm);
\draw (-2.5,1) ellipse (1.8 cm and 0.36cm);
\draw (-2.5,1) ellipse (1cm and 0.2cm);
\draw (-2.5,1) ellipse (0.8cm and 0.16cm);
\draw (2.5,1) ellipse (2cm and 0.4cm);
\draw (2.5,1) ellipse (1.8 cm and 0.36cm);
\draw (2.5,1) ellipse (1cm and 0.2cm);
\draw (2.5,1) ellipse (0.8cm and 0.16cm);
\draw (-2.5,0) ellipse (1.5cm and 0.3cm);
\draw (-2.5,0) ellipse (1.3cm and 0.26cm);
\draw (2.5,0) ellipse (1.5cm and 0.3cm);
\draw (2.5,0) ellipse (1.3cm and 0.26cm);
\draw (0,-1) ellipse (1.5cm and 0.3cm);
\draw (0,-1) ellipse (1.3cm and 0.26cm);
%%%%%%%%%%%%%%% top left half
\draw (-4.5,1) to[out=-90,in=90] (-4,0);
\draw (-3.3,1) to[out=-90,in=90] (-3.8,0);
\draw (-0.5,1) to[out=-90,in=90] (-1,0);
\draw (-1.7,1) to[out=-90,in=90] (-1.2,0);
\draw (-4.3,1)
  .. controls +(down:0.5cm) and +(down:0.5cm) .. (-3.5,1);
\draw (-0.7,1)
  .. controls +(down:0.5cm) and +(down:0.5cm) .. (-1.5,1);
%%%%%%%%%%%%%%% top right half
\draw (4.5,1) to[out=-90,in=90] (4,0);
\draw (3.3,1) to[out=-90,in=90] (3.8,0);
\draw (0.5,1) to[out=-90,in=90] (1,0);
\draw (1.7,1) to[out=-90,in=90] (1.2,0);
\draw (4.3,1)
  .. controls +(down:0.5cm) and +(down:0.5cm) .. (3.5,1);
\draw (0.7,1)
  .. controls +(down:0.5cm) and +(down:0.5cm) .. (1.5,1);
%%%%%% bottom half
%% vertical lines
\draw (-4,0)
  .. controls +(down:0.4cm) and +(up:0.2cm) .. (-1.5,-1);
\draw (4,0)
  .. controls +(down:0.4cm) and +(up:0.2cm) .. (1.5,-1);
\draw (-3.8,0)
  .. controls +(down:0.4cm) and +(up:0.2cm) .. (-1.3,-1);
\draw (3.8,0)
  .. controls +(down:0.4cm) and +(up:0.2cm) .. (1.3,-1);
%% inside
\draw (-1,0)
  .. controls +(down:0.3cm) and +(down:0.3cm) .. (1,0);
\draw (-1.2,0)
  .. controls +(down:0.5cm) and +(down:0.5cm) .. (1.2,0);
%% labels
\node at (-4.7,1) {$\overline{\VV}$};
\node at (-3.7,1) {$\overline{\WW}$};
\node at (0.3,1) {$\overline{\VV}'$};
\node at (1.3,1) {$\overline{\WW}'$};
\end{tikzpicture}
\]
}

\comment{
\[
\Skein (
\begin{tikzpicture}
\tikzmath{
  \ellx = 1;
  \elly = 0.2;
  \ellxs = 0.8;
  \ellys = 0.16;
}
\draw (-1.5,1) ellipse (\ellx cm and \elly cm);
\draw (-1.5,1) ellipse (\ellxs cm and \ellys cm);
\draw (1.5,1) ellipse (\ellx cm and \elly cm);
\draw (1.5,1) ellipse (\ellxs cm and \ellys cm);
\draw (0,-1) ellipse (\ellx cm and \elly cm);
\draw (0,-1) ellipse (\ellxs cm and \ellys cm);
%% outside lines
\draw (-2.5,1) to[out=-90,in=90] (-1,-1);
\draw (-2.3,1) to[out=-90,in=90] (-0.8,-1);
\draw (2.5,1) to[out=-90,in=90] (1,-1);
\draw (2.3,1) to[out=-90,in=90] (0.8,-1);
%% middle
\draw (-0.5,1) .. controls +(down:0.5cm) and +(down:0.5cm)
  .. (0.5,1);
\draw (-0.7,1) .. controls +(down:0.6cm) and +(down:0.6cm)
  .. (0.7,1);
%% labels
\node at (-1.5,1.4) {$\VV$};
\node at (1.5,1.4) {$\WW$};
\node at (0,-1.4) {$\mathbf{X}$};
\end{tikzpicture}
%%%%%%%%%%%%%%%%%%%%%%%%%%%%
)
=
\Skein (
%%%%%%%%%%%%%%%%%%%%%%%%%%%%
\begin{tikzpicture}
\tikzmath{
  \ellx = 1;
  \elly = 0.2;
  \ellxs = 0.8;
  \ellys = 0.16;
}
\draw (0,1) ellipse (\ellx cm and \elly cm);
\draw (0,1) ellipse (\ellxs cm and \ellys cm);
\draw (0,-1) ellipse (\ellx cm and \elly cm);
\draw (0,-1) ellipse (\ellxs cm and \ellys cm);
%% outside lines
\draw (-1,1) -- (-1,-1);
\draw (-0.8,1) -- (-0.8,-1);
\draw (1,1) -- (1,-1);
\draw (0.8,1) -- (0.8,-1);
%% labels
\node at (0,1.4) {$\VV \tnsr \WW$};
\node at (0,-1.4) {$\mathbf{X}$};
\end{tikzpicture}
)
\]
}
\comment{
Here we record several lemmas that are useful
for computations. We give no proofs,
referring readers to \ocite{stringnet},\ocite{KT}.

\begin{equation} \label{e:combine}
\begin{tikzpicture}
\node[small_morphism] (T) at (0,-0.4) {$\al$};
\node[small_morphism] (B) at (0,0.4) {$\al$};
\node at (0,1) {$\dots$};
\node at (0,-1) {$\dots$};
\draw[midarrow] (T)-- +(-120:0.8cm)
  node[pos=0.5,left] {\small $V_1$};
\draw[midarrow] (T)-- +(-60:0.8cm)
  node[pos=0.5,right] {\small $V_n$};
\draw[midarrow_rev] (B)-- +(120:0.8cm)
  node[pos=0.5,left] {\small $V_1$};
\draw[midarrow_rev] (B)-- +(60:0.8cm)
  node[pos=0.5,right] {\small $V_n$};
\draw[regular] (T) -- (B); 
\end{tikzpicture}
%%%%%%%%%%%%%%%%%
=
%%%%%%%%%%%%%%%%%
\begin{tikzpicture}
\node at (0,0) {$\dots$};
\draw[midarrow] (-0.3,1)-- (-0.3,-1)
  node[pos=0.5,left] {\small $V_1$};
\draw[midarrow] (0.3,1)-- (0.3,-1)
  node[pos=0.5,right] {\small $V_n$};
\end{tikzpicture}
\end{equation}

%%%%%%%%%%%%%%%%%%%%%%%%%%%%%%%%%%%
%%%%%%%%%%%%%%%%%%%%%%%%%%%%%%%%%%%

\begin{equation} \label{e:sliding}
\begin{tikzpicture}
\draw[regular] (0,0) circle(0.4cm);
\path[subgraph] (0,0) circle(0.3cm); 
\draw (0,1.2)..controls +(-90:0.8cm) and +(90:0.5cm) ..
  (-0.55, 0) ..controls +(-90:0.5cm) and +(90:0.8cm) ..
  (0,-1.2);
 \end{tikzpicture}
%%%%%%%%%%%%%
\quad=\quad
%%%%%%%%%%%%%
\begin{tikzpicture}
\draw[regular] (0,0) circle(0.4cm);
\node[small_morphism] (top) at (0,0.45) {\tiny $\al$};
\node[small_morphism] (bot) at (0,-0.45) {\tiny $\al$};
\path[subgraph] circle(0.3cm); 
\draw (0,1.2)--(top) (bot)--(0,-1.2);    
\end{tikzpicture}
%%%%%%%%%%%%%%
\quad=\quad 
%%%%%%%%%%%%%
 \begin{tikzpicture}
 \draw[regular] (0,0) circle(0.4cm);
 \path[subgraph] (0,0) circle(0.3cm); 
 \draw (0,1.2)..controls +(-90:0.8cm) and +(90:0.5cm) ..
   (0.55, 0) ..controls +(-90:0.5cm) and +(90:0.8cm) ..
   (0,-1.2);
 \end{tikzpicture}
\end{equation}
where the shaded region can contain anything.

%%%%%%%%%%%%%%%%%%%%%%%%%%%%%%%%%%%
%%%%%%%%%%%%%%%%%%%%%%%%%%%%%%%%%%%

\begin{equation} \label{e:al_natural}
\text{For }
f: V_1 \to W_1,\;\;\;\;
\begin{tikzpicture}
\node[small_morphism] (al) at (0,0) {$\al$};
\draw[->] (al)-- +(240:1cm) node[pos=0.7, left] {$V^{*}_1$} ;
\draw[->] (al)-- +(180:1cm);
\draw[->] (al)-- +(120:1cm);
\draw[->] (al)-- +(60:1cm);
\draw[->] (al)-- +(0:1cm);
\draw[->] (al)-- +(-60:1cm) node[pos=0.7, right] {$V^{*}_n$};
\end{tikzpicture}
\;\;\;\;
\begin{tikzpicture}
\node[small_morphism] (al) at (0,0) {$\al$};
\draw[->] (al)-- +(240:1cm) node[pos=0.7, left] {$V_n$} ;
\draw[->] (al)-- +(180:1cm);
\draw[->] (al)-- +(120:1cm);
\draw[->] (al)-- +(60:1cm);
\draw[->] (al)-- +(0:1cm);
\draw[midarrow={0.3},->] (al)-- +(-60:1cm) node[right] {$W_1$};
\node[small_morphism] at (-60:0.6cm) {\small $f$};
\end{tikzpicture}
%%%%%%%%%%%%%%%%%%%%%%%%%%%%%%%%%
=
%%%%%%%%%%%%%%%%%%%%%%%%%%%%%%%%%
\begin{tikzpicture}
\node[small_morphism] (be) at (0,0) {$\beta$};
\draw[midarrow={0.3},->] (be)-- +(240:1cm)
  node[left] {$V^{*}_1$} ;
\node[small_morphism] at (-120:0.6cm) {\tiny $f^*$};
\draw[->] (be)-- +(180:1cm);
\draw[->] (be)-- +(120:1cm);
\draw[->] (be)-- +(60:1cm);
\draw[->] (be)-- +(0:1cm);
\draw[->] (be)-- +(-60:1cm)
  node[pos=0.7,right] {$V^{*}_n$};
\end{tikzpicture}
\;\;
\begin{tikzpicture}
\node[small_morphism] (be) at (0,0) {$\beta$};
\draw[->] (be)-- +(240:1cm) node[pos=0.7, left] {$V_n$} ;
\draw[->] (be)-- +(180:1cm);
\draw[->] (be)-- +(120:1cm);
\draw[->] (be)-- +(60:1cm);
\draw[->] (be)-- +(0:1cm);
\draw[->] (be)-- +(-60:1cm) node[pos=0.7,right] {$W_1$};
\end{tikzpicture}
\end{equation}

\begin{equation} \label{e:charge_conservation}
\frac{1}{\cD}
\begin{tikzpicture}
\draw[midarrow={0.9}] (0,0) -- (0,-0.5);
\node at (0.15,-0.4) {\tiny $i$};
\draw[overline={1.5},regular] (0,0.1) circle (0.25cm);
\draw[overline={1.5}] (0,0) -- (0,0.5);
\end{tikzpicture}
=
\delta_{i,1} \id_{X_i}
\end{equation}
}
